# Supplementary material for: Generative AI Security: Challenges and Countermeasures
Source: arXiv:2402.12617 source file (2024-10-23)
Supplement: Supplementary file 1 [file appendix.tex]

\section{Additional Research Directions: Systematic Evaluation of GenAI Security}

A systematic approach to evaluating the security of GenAI systems is essential to understand and bolster their security comprehensively. Existing research has delved into various aspects of GenAI safety, including toxicity, susceptibility to jailbreaking and prompt injection, vulnerabilities in generated code, and resilience against misuse~\citep{wang2023decodingtrust, huang2023survey, toyer2023tensor, zhang2023safetybench, qiu2023latent}. Yet, there remain  a good amount of open problems for evaluation of GenAI security.

% Moreover, the current landscape necessitates a more encompassing and user-friendly framework that thoroughly characterizes all safety aspects of GenAI. This includes, but is not limited to, considerations such as function (API) calls for tool use, software manipulation, and the emergent risks associated with multi-modality in GenAI. Such a comprehensive assessment framework is vital for pinpointing vulnerabilities and steering the evolution of more secure GenAI systems. 
\begin{itemize}
\item \textbf{Defining the Safety Decision Boundary:} A crucial aspect of model development is understanding the delicate balance between helpfulness and harmlessness. Consider, for example, a model programmed to reject every query; while this ensures safety, it also renders the model ineffective in assisting users. Effective benchmark design necessitates a nuanced characterization of the safety decision boundary. This involves evaluating not just the safety aspects, but also preventing the model from being excessively cautious, to avoid an over-alignment that limits utility.

  \item \textbf{Scenario-Based Evaluation Methodology:} The implementation of scenario-based evaluations, simulating various real-world situations and potential threats, can yield more comprehensive insights into the practical security aspects of GenAI  systems. This method is instrumental in uncovering specific vulnerabilities that may remain hidden in theoretical assessments. The application of safety decision boundaries should vary based on the context of use. For instance, a cybersecurity analyst requiring knowledge of attack strategies for effective defense design should not be hindered by the model rejecting queries related to attack methodologies.

\item \textbf{Diversity and Interactivity in Evaluation:} We advocate for prioritizing the diversity  of attack methodologies as key criteria in benchmarks assessing GenAI security. This calls for a well-conceived design of interfaces that facilitate crowdsourcing. A notable example is Tensor Trust, which introduced an interactive framework for attack and defense simulations, providing a dynamic and engaging environment for evaluation.

% \dave{Feels abstract, I don't know what diverse or interactive means concretely or how to apply/measure it.}

\item \textbf{Applying Goodhart's Law to Benchmarking:} Goodhart's Law, succinctly expressed as "When a measure becomes a target, it ceases to be a good measure", is particularly relevant in the context of public benchmark datasets~\citep{strathern1997improving}. There's a risk of data contamination leading to training on the benchmark data, which can result in overfitting to a specific benchmark at the expense of overall safety and performance. The suitability of a fixed test set for language models is debatable, raising the intriguing challenge of how to develop an evolving test set or generate model-created test prompts, to counteract this issue~\citep{zou2023universal}.

\end{itemize}

% The overarching goal is to ensure that GenAI technologies are not only powerful and efficient but also safe, reliable, and trustworthy across various applications. This comprehensive and systematic approach to security evaluation is integral to achieving this goal.
 
% \banghua{Existing attempts. Decoding Trust paper. Shortcomings of existing ones. We don't have a safety benchmark. Tool-use security? Sth more specific. Problem statement.  }
